# Supplementary material for: TimeRewind: Rewinding Time with Image-and-Events Video Diffusion
Source: arXiv:2403.13800 source file (2024-03-20)
Supplement: Supplementary file 1 [file X_suppl.tex]

\section{Video Results}
\textbf{The supplementary material includes an  \textcolor{red}{HTML page  containing video results}.}
Please check the offline page for additional video results.

\section{Ablation Study}

In this section, we assess the impact of the number of learnable parameters in EMA module, the diversity of training sets, and the way of inserting the EMA module on the final performance of our backward-time video synthesis task.

\subsection{Impact of Number of Learnable Parameters in EMA Module}
